# Supplementary material for: BoxSplitGen: A Generative Model for 3D Part Bounding Boxes in Varying Granularity
Source: arXiv:2602.20666 source file (2026-02-24)
Supplement: Supplementary file 1 [file supplementary.tex]

% WACV 2026 Paper Template
% based on the ICCV 2025 template (https://media.eventhosts.cc/Conferences/ICCV2025/ICCV2025-Author-Kit-Feb.zip) with
% WACV-specific details (e.g., 2 tracks) from the WACV 2025 template (https://www.dropbox.com/scl/fi/su44zgdhrzik26p2xu37k/WACV-2025-Author-Kit-Template.zip?rlkey=5qcfimjhxnmx3wlyk7yhk8wg7&dl=0)

\documentclass[10pt,twocolumn,letterpaper]{article}

%%%%%%%%% PAPER TYPE  - PLEASE UPDATE FOR FINAL VERSION
\usepackage[wacv,algorithms]{wacv}      % To produce the REVIEW version for the algorithms track
% \usepackage[review,applications]{wacv}      % To produce the REVIEW version for the applications track
%\usepackage{wacv}              % To produce the CAMERA-READY version
%\usepackage[pagenumbers]{wacv} % To force page numbers, e.g. for an arXiv version

% Import additional packages in the preamble file, before hyperref
\input{preamble}

% It is strongly recommended to use hyperref, especially for the review version.
% hyperref with option pagebackref eases the reviewers' job.
% Please disable hyperref *only* if you encounter grave issues, 
% e.g. with the file validation for the camera-ready version.
%
% If you comment hyperref and then uncomment it, you should delete *.aux before re-running LaTeX.
% (Or just hit 'q' on the first LaTeX run, let it finish, and you should be clear).
\definecolor{wacvblue}{rgb}{0.21,0.49,0.74}
\usepackage[pagebackref,breaklinks,colorlinks,allcolors=wacvblue]{hyperref}

%%%%%%%%% PAPER ID  - PLEASE UPDATE
 % *** Enter the WACV Paper ID here

%%%%%%%%% TITLE - PLEASE UPDATE
\title{\Ours: A Generative Model for 3D Part Bounding Boxes in Varying Granularity --- Supplementary Material}

%%%%%%%%% AUTHORS - PLEASE UPDATE
\author{
Juil Koo\textsuperscript{$1\ast$} $\quad$
Wei-Tung Lin\textsuperscript{$2\ast$} $\quad$
% Minh Hieu Nguyen\textsuperscript{*} $\quad$
Chanho Park\textsuperscript{1}$\quad$
Chanhyeok Park\textsuperscript{1} $\quad$
Minhyuk Sung\textsuperscript{1} \\
\textsuperscript{1}KAIST$\quad$
\textsuperscript{2}NVIDIA\\
{\tt\small \{63days,charlieppark,chpark1111,mhsung\}@kaist.ac.kr
$\quad$
weitungl@nvidia.com}
% {\tt\small 63days@kaist.ac.kr$\quad$weitungl@nvidia.com$\quad$charlieppark@kaist.ac.kr$\quad$}\\
% {\tt\small chpark1111@kaist.ac.kr$\quad$mhsung@kaist.ac.kr}
}

\begin{document}

\onecolumn

\maketitle

\def\thefootnote{*}\footnotetext{Equal contribution.}\def\thefootnote{\arabic{footnote}}

%%%%%%%%%%%%%%%%%%%%%%%%%%%%%%%%%%%%%%%%%%%%%%%%%%%%%%%%%%%%

\appendix
\newif\ifarxiv
\arxivfalse
\input{sec/x_supp}

%%%%%%%%%%%%%%%%%%%%%%%%%%%%%%%%%%%%%%%%%%%%%%%%%%%%%%%%%%%%

\clearpage
% \newpage
% \newpage
{
    \small
    \bibliographystyle{ieeenat_fullname}
    \bibliography{main}
}

\end{document}
